# Supplementary material for: High-throughput Parasitic-independent Probe Thermal Resistance Calibration for Robust Thermal Mapping with Scanning Thermal Microscopy
Source: arXiv:2511.09960 ancillary file (2026-01-27)
Supplement: Supplementary file 1 [file Munde_JAP_Manuscript_SThM_2025_Supplementary.pdf]

Supplementary Material

# High-throughput Parasitic-independent Probe Thermal Resistance Calibration for Robust Thermal Mapping with Scanning Thermal Micrsocopy

Ram Munde,[1] Heng-Ray Chuang,[1] and Raisul Islam[1]
*Department of Materials Engineering, Purdue University, West Lafayette, USA*

(Dated: 13 November 2025)

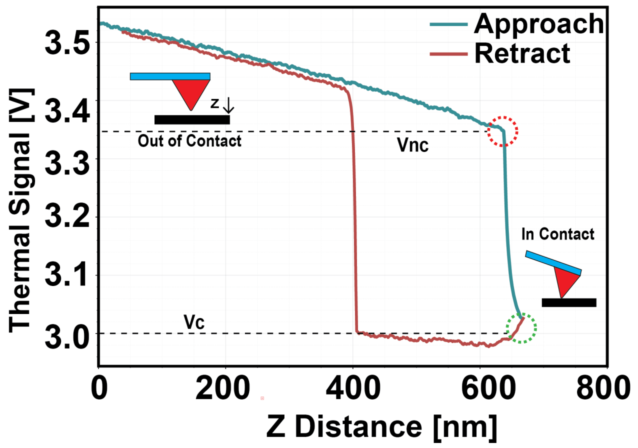


**Figure S. 1:** Thermal signals recorded during the approach–retract cycle of the SThM probe on the sample surface.

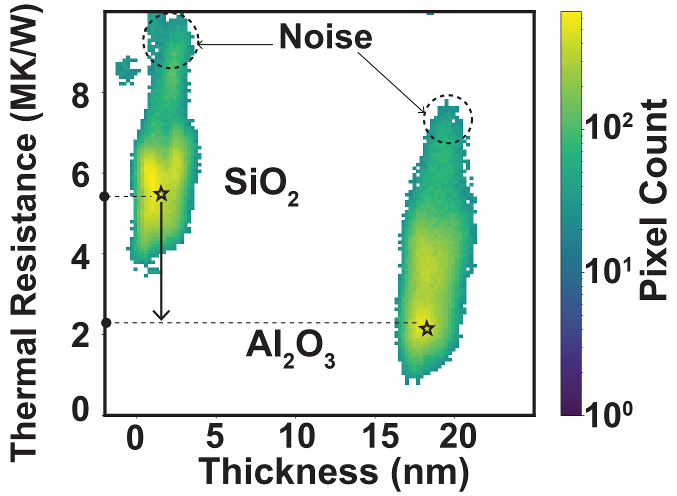


**Figure S. 2:** 2D Histogram of pixel-to-pixel correlation between the height and thermal resistance map.

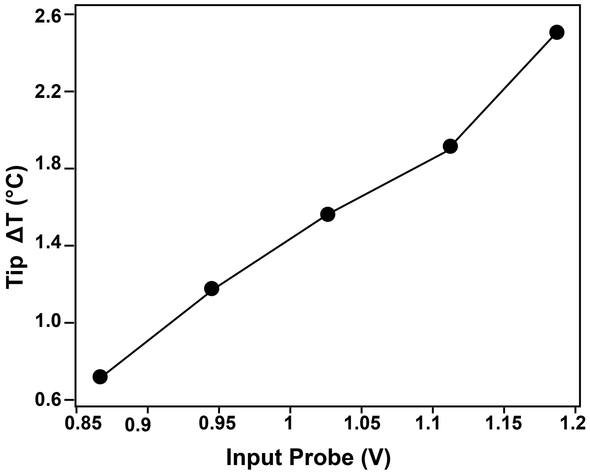


**Figure S. 3:** Calibration of the thermo-resistive probe for SThM. The resulting change in temperature ($\Delta T$) is calculated from the measured change in resistance ($\Delta R$) using the vendor-provided thermal coefficient of resistance (TCR), $\alpha$, which is defined as: $\Delta T \approx \frac{1}{R_0\alpha}\Delta R$ This calibration step establishes the critical relationship between the electrical signal (voltage/resistance) and the temperature of the probe tip, which is essential for converting raw SThM data into quantitative thermal map.

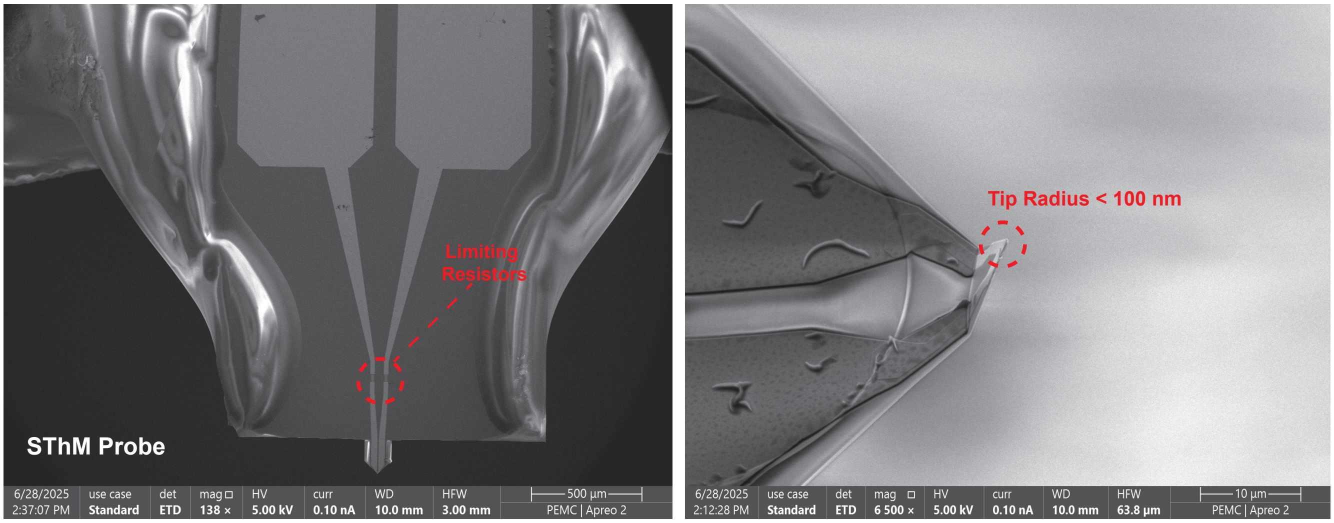


**Figure S. 4:** SEM images of SThM probe.

### S1. THERMAL CONDUCTIVITY AND UNCERTAINTY CALCULATION FOR $15\ nm$ ALUMINUM THIN FILM

The thermal conductivity of the Al film ($k_{Al}$) is determined using a differential method that compares the measured effective thermal resistance ($R$) of the film-on-substrate system ($R_{Al}$) against $SiO_2$ reference ($R_{SiO_2}$). A key simplification in this nanoscale measurement is the semi-infinite assumption for the $SiO_2$ substrate, which is validated because the substrate's 1.5 $\mu$m thickness ($L$) > probe tip radius ($b \sim 50$ nm), ensuring the thermal signal is contained and decoupled from the bottom boundary.

The known values are:

- Substrate thermal conductivity, $k_{SiO_2} = 1.38$ W/mK
- $SiO_2$ resistance, $R_{SiO_2} = 5.41 \pm 0.04$ MKW$^{-1}$

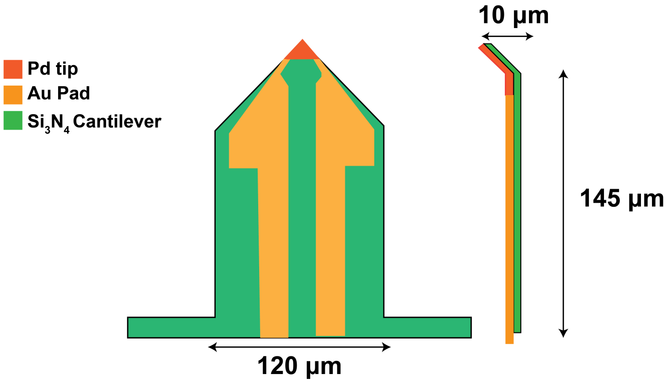


**Figure S. 5:** Geometry of SThM probe used in this study.

- Al film resistance, $R_{Al} = 2.60 \pm 0.03$ MKW$^{-1}$

$$k_{Al} = 1.38 \text{ W/mK} \times \left(\frac{5.41}{2.60}\right) \approx 2.8715 \text{ W/mK}$$

The total relative uncertainty ($\delta k_{\text{total}}/k$) is calculated by combining the measurement uncertainty and the $6\%$ additional uncertainty ($\delta_{\text{add}} = 0.06$) because of thermal signal consideration from water meniscus.

The relative uncertainty of the ratio $R_{\text{SiO}_2}/R_{Al}$ is:

$$\frac{\delta k_{\text{meas}}}{k} = \sqrt{\left(\frac{\delta R_{\text{SiO}_2}}{R_{\text{SiO}_2}}\right)^2 + \left(\frac{\delta R_{Al}}{R_{Al}}\right)^2} = \sqrt{\left(\frac{0.04}{5.41}\right)^2 + \left(\frac{0.03}{2.60}\right)^2} \approx 0.0137$$

$$\frac{\delta k_{\text{total}}}{k} = \sqrt{\left(\frac{\delta k_{\text{meas}}}{k}\right)^2 + (\delta_{\text{add}})^2} = \sqrt{(0.0137)^2 + (0.06)^2} \approx 0.0615$$

$$\delta k_{\text{total}} = 0.0615 \times 2.8715 \text{ W/mK} \approx 0.1767 \text{ W/mK}$$

$$k_{Al} = 2.87 \pm 0.18 \text{ W/mK}$$
